# Supplementary material for: A Generalized Linear Transport Model for Spatially-Correlated Stochastic Media
Source: arXiv:1410.8200 ancillary file (2014-10-29)
Supplement: Supplementary file 1 [file appendix_TTSP_Xu.pdf]

# Appendix A: Markov Chain Formalism for Generalized Radiative Transfer

For "literal" 1D RT ("$d$ = 1" in the main text), the plane-parallel medium becomes a finite line segment $[0,\tau^*]$ and each layer is bounded by two adjacent "nodes" on such a line. Accordingly, the phase function describes light scattering in only two possible directions: forward (with probability $p_+$) and backward (with probability $p_- = 1-p_+$). These probabilities are conveniently parameterized in Table 1 as $p_\pm = (1\pm g)/2$ where $g$ is the mean cosine of the scattering angle $\theta_s$, which is either +1 ($\theta_s = 0$) or –1 ($\theta_s = \pi$). Thus, $g = (+1)\text{x}p_+ + (-1)\text{x}p_-$ is between –1 and +1, and $g = 0$ (isotropic scattering ) leads to $p_+ = p_- = 1/2$.

To construct a computational Markov chain model, we discretize the medium into $N$ "layers" (sub-segments) so that each one has an optical thickness $\Delta\tau_n = \tau_n - \tau_{n-1}$ ($1 \le n \le N$) with $\tau_0 = 0$ and $\tau_N = \tau^*$. Moreover, we set the positive $\tau$-axis downward (or rightward, as in Fig. 3); that way, the solar source is at the upper (or left, as in Fig. 3) boundary at $\tau = \tau_0 = 0$.

Markov chain formalism, applied to computational RT in particular, describes a spatio-directional distribution of "particles" executing random walks *with no memory beyond the present state*. It has two key ingredients: (*i*) the initial distribution across all possible "states" (position on grid and direction of propagation), and (*ii*) the transition matrix, which describes the probability of a particle to jump from any given state to any other.

## A.1 Initial Light Distribution

The initial amount of light in the $n^{\text{th}}$ layer moving in direction $i = 0$ (downward) or $i = 1$ (upward) is created by a single scattering of the solar light that directly propagates from the upper boundary to the layer without suffering a collision. Assuming a uniform source of diffuse light in the layer, the first scattering redistributes (according to Bernoulli trial probabilities $p_\pm$) the solar light stopped in the layer through scattering.

Adopting conventional notation from Markov chain theory, we thus have the following fluxes in each direction ($i = 0,1$) per unit of optical distance:

$$\Pi_{0,(n,i)} = -F_0 \omega p(\Delta\theta_{i0}) \frac{1}{\Delta\tau_n} \int_{\tau_{n-1}}^{\tau_n} \dot{T}_a(\tau)\,\mathrm{d}\tau = -F_0 \omega p(\Delta\theta_{i0}) \frac{T_a(\tau_n) - T_a(\tau_{n-1})}{\Delta\tau_n}, \tag{A.1}$$

where $F_0$ is the incident flux at $\tau = 0$ (which we can assume is unity without loss of generality), $\omega$ is the single scattering albedo, $p(\Delta\theta_{i0})$ is the phase function, with $\Delta\theta_{i0}$ denoting the scattering angle formed between the incidence angle $\theta_0 = 0$ and the internal source angle $\theta_i$: $\Delta\theta_{i0} = |\theta_i - \theta_0|$. For downward propagation ($i = 0$), $\theta_i = 0$ and $\Delta\theta_{i0} = 0$ resulting in $p(\Delta\theta_{i0}) = p_+$, while for upward propagation ($i = 1$), $\theta_i = \pi$ and $\Delta\theta_{i0} = \pi$ resulting in $p(\Delta\theta_{i0}) = p_-$. Lastly, $T_a(\tau)$ denotes here the generalized transmission law in Eq. (34) of the main text, assuming unitary mean extinction ($\bar{\sigma} = 1$), while $-\dot{T}_a(\tau) > 0$ is the absolute value of its derivative, denoted $|\dot{T}_a(\tau)|$ in the main text. Recall that $T_a(\tau) = -\dot{T}_a(\tau) = \exp(-\tau)$ when $a = \infty$.

# A.2 Transition Matrix

The transition matrix **Q** (continuing to follow conventional notation from Markov chain theory) describes a particle's change from state $(n,i)$, meaning in layer $n$ and going in direction $i$, into another state $(n',j)$. Imagine light traveling from the $n^{\text{th}}$ to $n'^{\text{th}}$ layer, extinguished in the $n'^{\text{th}}$ layer in its original direction $i$, and is then scattered into the new direction $j$. Each element $Q_{(n',j),(n,i)}$ of **Q** quantifies the probability of such a change:

$$Q_{(n',j),(n.i)} = \begin{cases} -\dfrac{1}{\Delta\tau_n} \displaystyle\int_{\tau_{n-1}}^{\tau_n} \int_{\tau_{n'-1}}^{\tau_{n'}} \dot{T}_a(\tau - x)\omega p(\Delta\theta_{ji})\,\mathrm{d}x\,\mathrm{d}\tau, & n > n' \\ (1 - P_{\text{esc}})\omega p(\Delta\theta_{ji}), & n = n' \\ -\dfrac{1}{\Delta\tau_n} \displaystyle\int_{\tau_{n-1}}^{\tau_n} \int_{\tau_{n'-1}}^{\tau_{n'}} \dot{T}_a(x - \tau)\omega p(\Delta\theta_{ji})\,\mathrm{d}x\,\mathrm{d}\tau, & n < n' \end{cases}, \tag{A.2}$$

where $\Delta\theta_{ji} = |\theta_j - \theta_i|$ is the scattering angle and the average escaping probability of a particle leaving $n^{\text{th}}$ layer is

$$P_{\text{esc}} = \frac{1}{\Delta\tau_n} \int_0^{\Delta\tau_n} T_a(\tau)\,\mathrm{d}\tau\ . \tag{A.3}$$

Note in (A.2) the finite probability in the discrete world of the particle remaining in the same layer. Eq. (A.2) is evaluated analytically. For $n > n'$:

$$Q_{(n',j),(n.i)} = -\omega p(\Delta\theta_{ji})\frac{1}{\Delta\tau_n}\int_{\tau_{n-1}}^{\tau_n}\int_{\tau_{n'-1}}^{\tau_{n'}}\dot{T}_a(\tau - x)\,\mathrm{d}x\,\mathrm{d}\tau$$

$$= -\omega p(\Delta\theta_{ji})\frac{1}{\Delta\tau_n}\int_{\tau_{n-1}}^{\tau_n}\left[T_a(\tau-\tau_{n'-1}) - T_a(\tau-\tau_{n'})\right]\mathrm{d}\tau$$

$$= -\omega p(\Delta\theta_{ji})\frac{1}{\Delta\tau_n}\left\{\left[F(\tau_n,\tau_{n'-1}) - F(\tau_{n-1},\tau_{n'-1})\right] - \left[F(\tau_n,\tau_{n'}) - F(\tau_{n-1},\tau_{n'})\right]\right\}$$

(A.4)

where

$$F(\tau,x) = \int T_a(\tau - x)\,\mathrm{d}\tau = \begin{cases}\ln(\tau - x + 1), & a = 1\\ -\dfrac{a}{a-1}\left[\dfrac{\tau - x}{a} + 1\right]^{-(a-1)}, & a \neq 1\end{cases} \quad \text{(A.5)}$$

including $-\exp[-(\tau - x)]$ when $a = \infty$. For $n < n'$:

$$Q_{(n',j),(n.i)} = -\omega p(\Delta\theta_{ji})\frac{1}{\Delta\tau_n}\int_{\tau_{n-1}}^{\tau_n}\int_{\tau_{n'-1}}^{\tau_{n'}}\dot{T}_a(x - \tau)\,\mathrm{d}x\,\mathrm{d}\tau$$

$$= -\omega p(\Delta\theta_{ji})\frac{1}{\Delta\tau_n}\left\{\left[F(\tau_{n'-1},\tau_n) - F(\tau_{n'-1},\tau_{n-1})\right] - \left[F(\tau_{n'},\tau_n) - F(\tau_{n'},\tau_{n-1})\right]\right\}.$$

(A.6)

Finally, for $n = n'$:

$$Q_{(n',j),(n.i)} = \omega p(\Delta\theta_{ji})(1 - P_{\mathrm{esc}}) = \omega p(\Delta\theta_{ji})\frac{1}{\Delta\tau_n}\left\{\Delta\tau_n - \left[F(\Delta\tau_n,0) - F(0,0)\right]\right\},$$

(A.7)

where $F(0,0) = 0$ for $a = 1$, and $-a/(a-1)$ for $a \neq 1$ ($-1$ when $a = \infty$).

# A.3 Markov Chain Model

With the initial light distribution vector $\mathbf{\Pi}_0$ and transition matrix $\mathbf{Q}$, multiple light scattering processes in the spatially-correlated stochastic medium with a general (exponential or not) transmission law or propagation kernel can be expressed in the form of a matrix series, namely,

$$\mathbf{\Pi}_{\mathrm{tot}} = \mathbf{\Pi}_0 + \mathbf{Q}\mathbf{\Pi}_0 + \mathbf{Q}\mathbf{Q}\mathbf{\Pi}_0 + \ldots = (\mathbf{E} - \mathbf{Q})^{-1}\mathbf{\Pi}_0, \quad \text{(A.8)}$$

where $\mathbf{E}$ is the identity matrix, and $\mathbf{\Pi}_0$, $\mathbf{Q\Pi}_0$, $\mathbf{QQ\Pi}_0$, … represent the contributions from first, second, third, and higher orders of scattering, respectively.

The total diffusely reflected ($R_{\text{dif}}$) and transmitted ($T_{\text{dif}}$) light are contributed by different layers, namely,

$$F_0 R_{\text{dif}} = I_{\text{dif, up}}^{\text{top}} = \sum_{n=1}^{N} \Pi_{\text{tot},(n,1)} \bar{T}_a(n,0) \Delta\tau_n \,, \tag{A.9}$$

$$F_0 T_{\text{dif}} = I_{\text{dif, dn}}^{\text{bot}} = \sum_{n=1}^{N} \Pi_{\text{tot},(n,0)} \bar{T}_a(n,\tau^*) \Delta\tau_n \,, \tag{A.10}$$

at the top and bottom of medium, respectively. For consistency with the assumption of uniform source distribution in every layer, an average transmission is used for the particles leaving the $n^{\text{th}}$ layer for a given location $x$ in the medium, namely,

$$\bar{T}_a(n,x) = \begin{cases} \dfrac{1}{\Delta\tau_n} \displaystyle\int_{\tau_{n-1}}^{\tau_n} T_a(\tau - x)\,\mathrm{d}\tau, & x \le \tau_{n-1} \\ \dfrac{1}{\Delta\tau_n} \displaystyle\int_{\tau_{n-1}}^{\tau_n} T_a(x - \tau)\,\mathrm{d}\tau, & x \ge \tau_n. \end{cases} \tag{A.11}$$

Invoking Eq. (A.5), the above expressions become

$$\bar{T}_a(n,x) = \begin{cases} \dfrac{1}{\Delta\tau_n} \left[ F(\tau_n, x) - F(\tau_{n-1}, x) \right], & x \le \tau_{n-1} \\ -\dfrac{1}{\Delta\tau_n} \left[ F(x, \tau_n) - F(x, \tau_{n-1}) \right], & x \ge \tau_n. \end{cases} \tag{A.12}$$

Finally, to compute the diffuse intensity field at the top and bottom of the $n^{\text{th}}$ layer, (A.9)–(A.10) should be generalized to

$$I_{\text{dif,up}}^{(n)} = \sum_{k=n}^{N} \Pi_{\text{tot},(k,1)} \bar{T}_a(k, \tau_{n-1}) \Delta\tau_n \,, \tag{A.13}$$

$$I_{\text{dif,dn}}^{(n)} = \sum_{k=1}^{n} \Pi_{\text{tot},(k,0)} \bar{T}_a(k, \tau_n) \Delta\tau_n \,. \tag{A.14}$$

Sums $J$ and differences $F$ of these quantities, as defined from (45)–(46), are plotted in Fig. 3 for a variety of parameters $\{\omega, g, a\}$ when $\tau^* = 10$.

## A.4 Energy Conservation

We have the following energy conservation when $\omega = 1$ (no absorption), after including the directly transmitted light $T_a(\tau^*)$:

$$R_{\text{dif}} + T = R_{\text{dif}} + [T_{\text{dif}} + T_a(\tau^*)] = 1. \tag{A.15}$$

This identity was used as a first verification test for the Markov chain code. Other tests are described in §4.3 of the main text.

## A.5 Relation to Quantities and Methods Used in Main Text

The way the above formulation of the literal 1D RT problem is derived from the first principles of Markov chain theory is interesting because we arrive immediately at the Neumann series solution of a discrete version of the ancillary integral form of the RTE for $d = 1$, namely, Eq. (53) in the main text.

Indeed, the large-but-finite state vector $\mathbf{\Pi}_{\text{tot}}$ is nothing more than a discrete version of the source function $S_\pm(\tau)$ as can be seen already by comparing (A.1) for its initial value $\mathbf{\Pi}_0$ and the source term $Q_{S\pm}(\tau)$ in Eq. (54), paying attention to definitions rather than to notations. Consequently, the large system of coupled linear equations that is solved in (A.8), namely, $\mathbf{\Pi}_{\text{tot}} = \mathbf{Q}\mathbf{\Pi}_{\text{tot}} + \mathbf{\Pi}_0$, is nothing more than a discrete version of the generalized ancillary integral RTE in Eq. (53), solved formally in Eq. (55). The transition matrix $\mathbf{Q}$ is therefore just a discretized version of the kernel $K_S(\tau',\pm';\tau,\pm)$ for that integral equation, written out explicitly in Eq. (53). Finally, boundary-leaving and internal radiances are obtained from the known $\mathbf{\Pi}_{\text{tot}}$ with (A.9)–(A.10) and (A.13)–(A.14) respectively. These are simply the discrete-space counterparts of the formal solution of the 1D RTE, as used in generalized RT to compute $I_\pm(\tau)$ from $S_\pm(\tau)$, once it is a known quantity; its expression for $d = 1$ can be seen in Eq. (56).

Before closing, it is important to recall that the Monte Carlo method in linear transport/RT theory is put on a solid mathematical footing using the same Markov chain concepts as used here [65]. Finally, we recall that the key assumption in our *generalized* RT theory is to modify all the spatial integral expressions without requiring that there be a differential formulation from which they are normally derived.
